# Supplementary material for: Gaps in Topological Magnon Spectra: Intrinsic vs. Extrinsic Effects
Source: arXiv:2204.03720 source file (2022-04-07)
Supplement: Supplementary file 1 [file Supplemental.pdf]

# Supplemental material for "Gaps in Topological Magnon Spectra: Intrinsic vs. Extrinsic Effects"


Seung-Hwan Do,[1] Joe A. Paddison,[1] Gabriele Sala,[2] Travis J. Williams,[3] Koji Kaneko,[4,5] Keitaro Kuwahara,[6] A. F. May,[1] Jiaqiang Yan,[1] Michael A. McGuire,[1] Matthew B. Stone,[3] Mark D. Lumsden,[3] and Andrew D. Christianson[1]

[1]*Materials Science and Technology Division, Oak Ridge National Laboratory, Oak Ridge, Tennessee 37831, USA*
[2]*Second Target Station, Oak Ridge National Laboratory, Oak Ridge, Tennessee 37831, USA*
[3]*Neutron Scattering Division, Oak Ridge National Laboratory, Oak Ridge, Tennessee 37831, USA*
[4]*Materials Sciences Research Center, Japan Atomic Energy Agency, Tokai, Ibaraki 319-1195, Japan*
[5]*Advanced Science Research Center, Japan Atomic Energy Agency, Tokai, Ibaraki 319-1195, Japan*
[6]*Institute of Quantum Beam Science, Ibaraki University, Mito, Ibaraki 310-8512, Japan*


## I. EXPERIMENTAL DETAILS AND SPECTRAL SIMULATION METHODS

A single piece of $CrCl_3$ single crystal (mass: 0.88g and dimension: $12 \times 12 \times 4$ mm$^2$) was aligned with $[H,K,0]$ in the horizontal scattering plane for the inelastic neutron scattering (INS) measurements (see Fig. S1(a)). The sample was sealed within an aluminum can under an atmosphere of helium exchange gas at room temperature. Figure S1(b) and (c) show the elastic scattering for the $(H,K,1)$ and $(H,0,L)$ planes. Sharp magnetic reflections appear as magnetic satellite peaks with the ordering wave vector $\boldsymbol{Q}_\mathbf{m} = (0,0,\frac{3}{2})$ in the $R\bar{3}$ rhombohedral crystal structure, representing the alternative magnetic stacking order of the ferromagnetic honeycomb lattice. The rocking scan for $\boldsymbol{Q}= (3,0,0)$ Bragg reflection was fitted with a Gaussian function, as shown in Fig. S1(d), which gives the full-width at half-maximum (FWHM) $\sim 0.68°$, indicating the sample mosaicity is smaller than $\sim 0.68°$.

The INS data were obtained at $T = 5$ K using the SEQUOIA time-of-flight spectrometer located at the Oak Ridge National Laboratory (ORNL). The Fermi chopper was set to 120 Hz, 180 Hz, and 240 Hz for $E_\mathrm{i} = 4$, 11, and 25 meV, which give FWHM= 0.11, 0.24, and 0.65 meV of resolution at the elastic line ($E$=0 meV), respectively. For $E_\mathrm{i} = 25$ meV, measurements were performed by rotating the sample through 180° about its vertical axis with 0.5° steps. For $E_\mathrm{i} = 11$ meV, measurements were performed by rotating the sample $2*50°$ with 1° step covering two K-points at $(-1,2,0)$ and $(2,-1,0)$ (see Fig. S2(a)). The $E_\mathrm{i} = 4$ meV data was measured by rotating the sample through 35° about its vertical axis to cover $\boldsymbol{Q}$ along the $[H,0,0]$-direction. Data were reduced and analyzed using the Mantid [1], Dave [2], and Horace [3] software packages.

Spin-wave spectra were calculated using the SpinW package [4]. In comparison to measured spectra, the orthogonal integration range d$Q$ was accounted for by averaging over the resolution convoluted $\boldsymbol{Q}$-$E$ spectra at $\sim 10$ $Q$-points per 0.01Å$^{-1}$ within the range. The triple-axis spectroscopy simulations shown in Fig.4(c)(d) of the main text were performed using ResLib [5] with the resolution function calculation using the Popovici method [6] using the experimental parameters of the IN8 spectrometer used in Ref.[7].

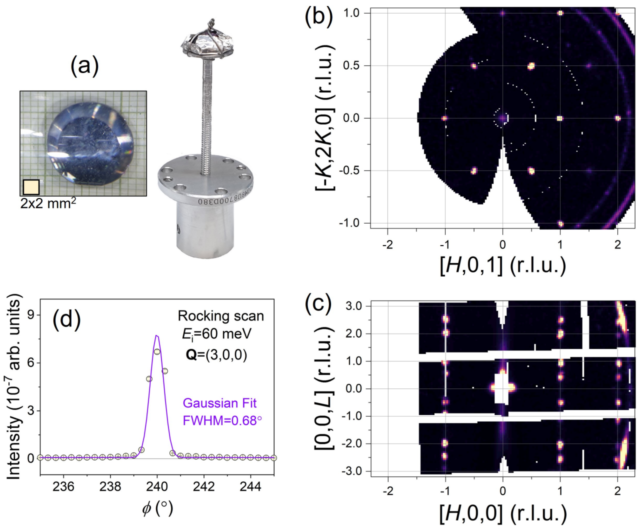


FIG. S1. (a) A picture of aligned $CrCl_3$ single crystal used for INS measurements. Elastic scattering for (b) $[H,K,1]$ and (c) $[H,0,L]$ were obtained from SEQUOIA using $E_\mathrm{i} = 25$ meV. Nuclear reflections appear at $-H+K+L = 3m$ ($m$ =integer) with reverse-obverse twins for $R\bar{3}$ structure. Magnetic reflections appear with a propagation vector $\boldsymbol{Q}_\mathrm{m} = (0,0,\frac{3}{2})$. The ring-patterns are scattering from the aluminum sample holder. (d) A rocking scan for the Bragg reflection at $\boldsymbol{Q}= (3,0,0)$ using $E_\mathrm{i} = 60$ meV. The solid line is the Gaussian fit to the data.

## II. DATA SYMMETRIZATION AND CONFIRMATION OF GAPLESS DIRAC MAGNON

While unsymmetrized data was used for $E_\mathrm{i} = 25$ meV to analyze the linear spin-wave theory and to make figures shown in the main text, $E_\mathrm{i} = 11$ meV and 4 meV data were symmetrized using symmetry operations of the Laue class of the $R\bar{3}$ to enhance statistics. Figure S2 shows a comparison between unsymmetrized and symmetrized data for $E_\mathrm{i} = 11$ meV. The shown magnon spectra in the symmetrized data exhibits the same $\boldsymbol{Q}$-$E$ pattern as the unsymmetrized data, but the signal to noise ratio is improved.

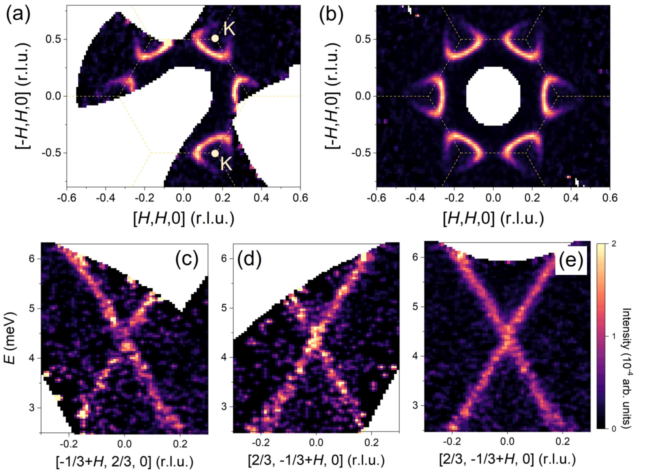


FIG. S2. Comparison of INS data for $E_\mathrm{i}$=11 meV with and without symmetrization. (a) The unsymmeterized constant energy slice data for $E=[2.85,3.15]$ meV and (b) corresponding symmetrized data. Unsymmetrized transverse $\boldsymbol{Q}$-scans for the two K-points at (c) $\boldsymbol{Q}$=$(-\frac{1}{3},\frac{2}{3},0)$ and (d) $\boldsymbol{Q}$=$(\frac{2}{3},-\frac{1}{3},0)$ and (e) corresponding symmetrized data at $(\frac{2}{3},-\frac{1}{3},0)$ were obtained by integrating over $\mathrm{d}Q^{\mathrm{rad}}=\pm0.01$ and $-2.5\leq L\leq 2.5$.

## III. SPIN-WAVE FITTING RESULTS AND DETERMINATION OF THE HAMILTONIAN PARAMETERS

Experimental dispersions were extracted by fitting Gaussian functions to the constant momentum scans for $E_\mathrm{i}=25$ meV and 11 meV data along the high symmetry directions (see Fig. S3(b)). 570 dispersion points were obtained from the both $E_\mathrm{i}=11$ and 25 meV energy spectra (filled circles in Fig. S3(c)), and used for fitting the spin-wave dispersions for the spin Hamiltonian model [Fig. S3(c)],

$$\mathscr{H}_0 = J_1\sum_{ij}S_iS_j + J_2\sum_{ij}S_iS_j + J_3\sum_{ij}S_iS_j + J_{\mathrm{int}}\sum_{ij}S_iS_j - D^z\sum_i (S_i^z)^2. \quad (1)$$

This Hamiltonian model describes Heisenberg exchanges up to third nearest neighbor (n.n.) interactions ($J_\mathrm{n}$) in a honeycomb layer, Heisenberg n.n. inter-layer interaction ($J^{\mathrm{int}}$) along $c$-axis, and easy-plane single-ion anisotropy ($D^z>0$) (see Fig. S3(a) for the exchange paths). Due to the highly two-dimensional magnon spectra, out-of-plane spin interactions were assumed to be negligible and for simplicity $J_{\mathrm{int}}=0.001$ meV was used to stabilize the antiferromagnetic layer order (see below for sensitivity of the $\chi^2$ on $J_{\mathrm{int}}$).

For fitting the spin-wave dipsersion, the $\chi^2$ optimization function was defined as following,

$$\chi^2 = \frac{1}{n}\sum_i \frac{(E_i^{obs}-E_i^{calc.})^2}{\sigma_i^2}, \quad (2)$$

where $E_i^{\mathrm{obs}}$ and $E_i^{\mathrm{calc}}$ indicate observed and calculated dispersion energies, and $n$ and $\sigma_\mathrm{i}$ indicate the number of dispersion points and standard deviation in the observed dispersion. The fitting of the Hamiltonian parameters to minimize the $\chi^2$ was performed using the algorithm implemented in the SpinW package [4]. The comparison of the calculated dispersion for the optimized parameters to experimental dispersion is shown in Fig. S3(c), and shows a good agreement. In addition, Fig. S3(d) shows a comparison of the extracted magnon scattering intensity with the spin-wave calculation: the good agreement indicates the existence of isotropically or randomly

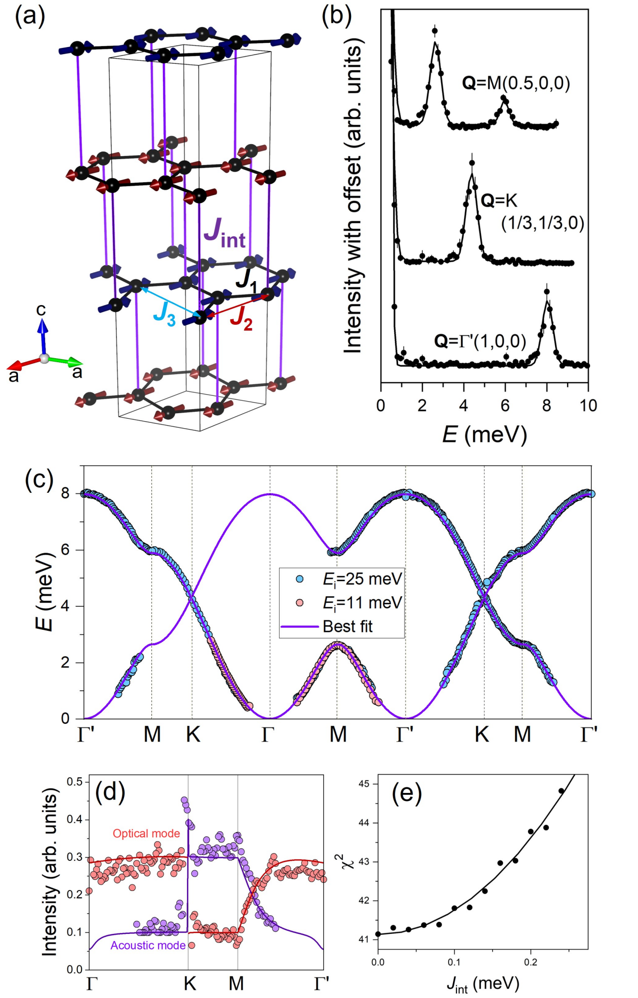


FIG. S3. (a) Magnetic structure and exchange paths for $CrCl_3$. Ferromagnetic moments are aligned in the $ab$-plane and antiferromagnetically stacked along the $c$-axis. The exchange paths are labeled. (b) Constant momentum scans at the high symmetry points in the Brillouin zone (dots). The black solid lines indicate the Gaussian fitting results on the elastic ($E=0$) and inelastic ($E\neq0$) excitation peaks. (c) Comparison between experimental dipersion points from $E_\mathrm{i}=25$ meV (blue filled circles) 11 meV (pink filled circles) and calculated dispersion (solid purple line) from the best fitting result. (d) Extracted intensity of acoustic (violet dot) and optical (red dot) modes and comparison to LSWT calculation (solid lines). The black arrow indicates the intensity at the K-point. (e) The $\chi^2$ value as a function of the $J_{\mathrm{int}}$ interaction strength. The black solid line indicates the parabolic fitting result.

distributed magnetic domains in the plane without preferred orientation.

To check the sensitivity of the inter-layer interaction to the obtained parameters, Fig. S3(e) shows the $\chi^2$ values of the dispersion points as a function of the $J_{\rm int}$ interaction strength with fixed other parameters. The antiferromagnetic interaction was only considered to stabilize the alternative stacking order ground state. The minimum $\chi^2$ appears near $J_{\rm int}$ $\sim$0 meV, and the $\chi^2$ shows parabolic increase with increasing $J_{\rm int}$. The graphical errobar estimation on the local $\chi^2$ minimum gives the error of $J_{\rm int}$ with $\sim 0.13$ meV [8], corresponding to the sensitivity of the parameter on the spin-wave fitting result. Due to the small number of interaction paths for $J_{\rm int}$ (number of interactions on a single spin: $\#J_{\rm int} = 1$) [Fig. S3], the spin-wave can be less-sensitive to varying the $J_{\rm int}$, compared to other exchanges paths for fixed values of exchange ($\#J_1 = 3$, $\#J_2 = 6$, and $\#J_3 = 3$).

## IV. LOW ENERGY MAGNON SPECTRA: GAPLESS DISPERSION AT Γ-POINT AND DISPERSION-LESS SPIN-WAVE ALONG *L*

The low-energy spectra near the zone center (ZC) shown in Fig. S4(a) reveals a quadratic dispersion as expected for a ferromagnetic spin-wave, $E \propto A\boldsymbol{Q}^2 + \Delta_\Gamma$, where $A$ and $\Delta_\Gamma$ are the spin-wave stiffness and magnon gap at the ZC. The low-energy magnon dispersion for energy transfers less than 1.2 meV, measured in the $E_{\rm i}$=4 meV configuration, were fitted with the function, which yields $A$=17.14(49) and $\Delta_\Gamma$=0.00(1) meV. The resulting gapless (Goldstone) mode ($\Delta_\Gamma$ $\sim$0 meV) indicates the preserved U(1) symmetry of Cr spins. This gapless feature is in contrast to the other chromate trihalide materials [9, 10], which emphasizes the importance of the ligand atom's SOC in determining the magnetic anisotropy of the systems [11]. Figure S4(b) shows no discernible dispersion along $[0.12, 0, L]$ near the ZC. Also, no dispersion along $[0, 0, L]$ through the ZC is detected within instrumental resolution (FWHM= 0.24 meV at $E = 0$ meV for $E_{\rm i} = 11$ meV) [Fig S4(c)]. The bandwidth along the $L$-direction is smaller than the instrumental resolution $W_L <$ FWHM/2 $\sim 0.12$ meV, corresponding to less than 1.5% of $W_{HK}$, indicating highly two-dimensional spin interactions in $CrCl_3$.

## V. DIRAC MAGNON ALONG THE RADIAL DIRECTION

In this section, we investigate the Dirac magnon spectra along a radial direction through the K-point with different orthogonal $\boldsymbol{Q}$-integration ranges $\mathrm{d}Q^{\rm trans} = \pm 0.05$ r.l.u. and $\pm 0.2$ r.l.u. (see Fig.2(b) in the main text for definition of $\mathrm{d}Q^{\rm trans}$). These $\mathrm{d}Q^{\rm trans}$ values are typical $Q$-integration ranges that were used for Ref. [7, 12]. Figure S5 shows the magnon spectra along the $[2H, -H, 0]$-direction (equivalent direction to the $[H, H, 0]$-direction) for the different $\mathrm{d}Q^{\rm trans}$ sizes. As the $\mathrm{d}Q^{\rm trans}$ increases, the magnon dispersion appears to open a gap at the K-point, $(\frac{2}{3}, -\frac{1}{3}, 0)$: while the constant momentum scan for $\mathrm{d}Q^{\rm trans}$=0.01, the data for $\mathrm{d}Q^{\rm trans} = \pm 0.05$ shows two

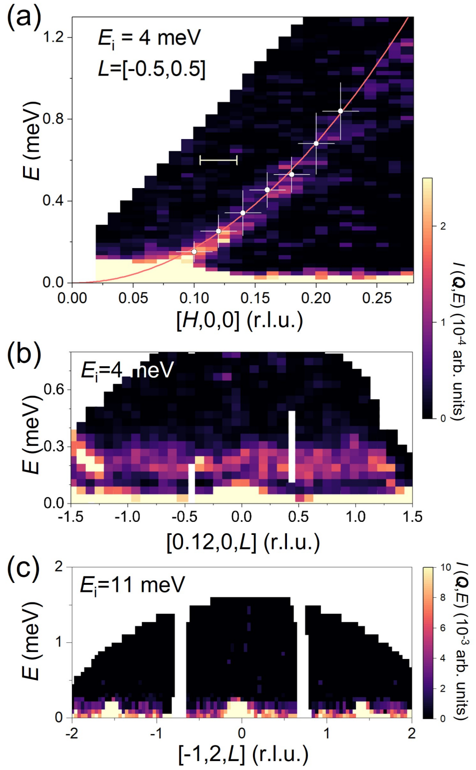


FIG. S4. (a) Low-energy spectrum near the magnetic zone center at Γ $(0, 0, 0)$ along $[H, 0, 0]$. The low-energy dispersion points and its energy line-widths were extracted by Gaussian fits to the constant momentum scans and are exhibited as points with vertical error-bars. The horizontal error-bars indicate integration range for the constant momentum scans. Solid line indicates a gapless biquadratic ferromagnetic spin-wave dispersion, $E \propto A\boldsymbol{Q}^2$+$\Delta_\Gamma$. (b) Magnon spectra along $[0.12, 0, L]$ with integration range marked by the bar in (a). (c) Low-energy spectrum near the magnetic zone centers at $\boldsymbol{Q}$=$(-1, 2, -\frac{3}{2})$, $(-1, 2, 0)$, and $(-1, 2, \frac{3}{2})$ along $[0, 0, L]$.

separated peaks with gap $\Delta_{\rm K} \sim 0.5$ meV. The measured spectra were compared to the spin-wave calculations for the determined Hamiltonian parameters in the Fig. S5(d)(e), and the observed gapless and gaped spectra for $\mathrm{d}Q^{\rm trans} = \pm 0.01$ and $\pm 0.05$ are closely reproduced by the pure Heisenberg model ($J_1 - J_2 - J_3$ model). These results confirm that the orthogonal integration range for the radial $\boldsymbol{Q}$-direction produces an extrinsic gap, same as the transverse direction discussed in the main text.

On the other hand, the momentum integration range $\mathrm{d}Q^{\rm trans} = \pm 0.2$ covers nearly half of the Brillouin zone, and the obtained spectra may not reflect the localized spectrum near the K-point. Thus, the shown spectra in Fig. S5(c) and (f) show a very broadened excitation due to the widely averaged spectral weight of the acoustic and optical modes. Accordingly, the constant momentum scan shows two broad peaks with a separation of $\sim 3$ meV for the gapless spin-wave model, which represents spectral centers of the averaged acoustic and optical modes' spectral weights, not corresponding to the Dirac magnon gap. Therefore, such a large momentum in-

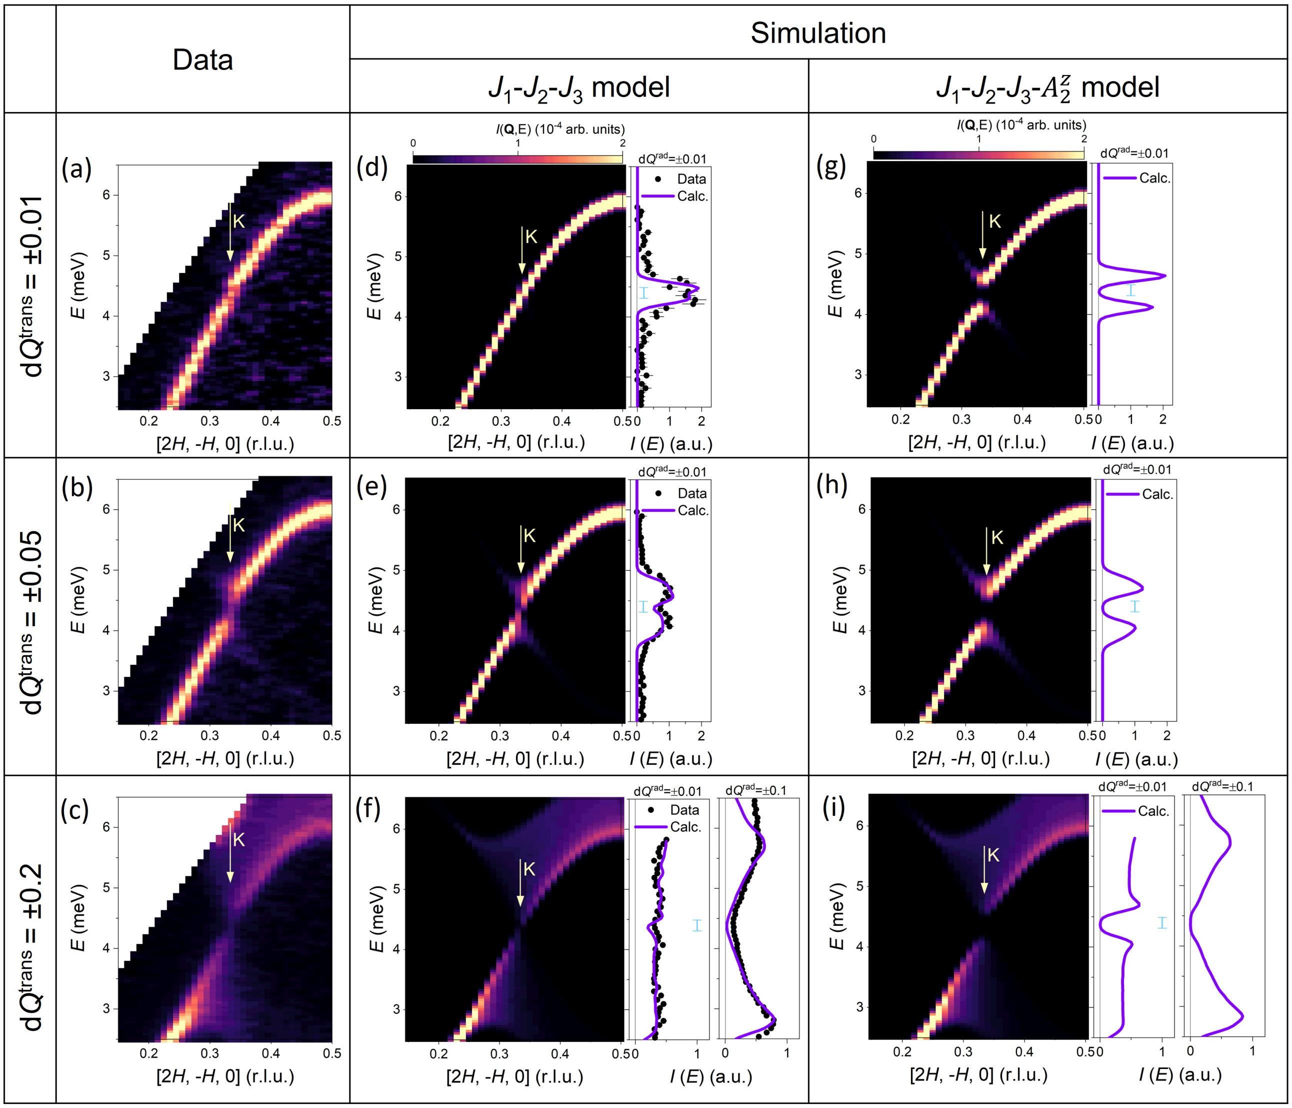


FIG. S5. Dependence of the apparent scattering at the Dirac point along radial $\boldsymbol{Q}$-direction on the range of momentum integration. (a-c) The INS spectra were measured using high resolution mode with $E_\text{i} = 11$ meV with the SEQUOIA spectrometer, with varying the orthogonal momentum integration range $dQ^\text{trans} = \pm 0.01$, 0.05, and 0.2 r.l.u. (0.012, 0.061 0.244Å$^{-1}$, respectively) and $-2.5 \leq L \leq 2.5$ r.l.u.. The spin-wave spectra were calculated for the determined Hamiltonian of the $J_1 - J_2 - J_3$ model(d-f) and the $J_1 - J_2 - J_3 - A_2^z$ model (g-i) with the identical $Q$-integration ranges. Blue bars in the figure indicate the instrumental resolution at $E^\text{Dirac}$.

tegration range should not be used to investigate the Dirac magnon spectra.

To compare the observed apparent gap with an intrinsic magnon gap arising from the well-known topological magnon example, we assumed a ferromagnetic spin structure aligned along the $c$-axis, same as in the $CrBr_3$, $CrI_3$, and $CrMTe_3$ (M=Si,Ge), and introduced the second n.n. DMI ($A_2^z$) along the $z$-axis to the original spin Hamiltonian model ($\mathscr{H}_0$). Then, the new Hamiltonian ($\mathscr{H}_1$) is

$$\mathscr{H}_1 = \mathscr{H}_0 + \sum_{ij} A_2^z \cdot (S_i \times S_j). \quad (3)$$

Here we considered $A_2^z = J_2 = 0.03$ meV, corresponding to $\sim$3% of $J_1$, and the resulting spin-wave calculations are exhibited in Fig. S5(g-i). The DMI breaks the time-reversal symmetry of magnon, which results in a clear peak splitting from an *intrinsic* gap for all the orthogonal $\boldsymbol{Q}$ integration values [13]. Noticeably, this intrinsic magnon gap features almost zero scattering intensity at the $E^\text{Dirac}$ regardless of the size of the momentum integration range, in contrast to the pure Heisenberg $J_1 - J_2 - J_3$ model. This further indicates how the intrinsic gap and the spurious gap can appear differently in the measured spectra where energy resolution is sufficiently smaller than the intrinsic magnon gap.

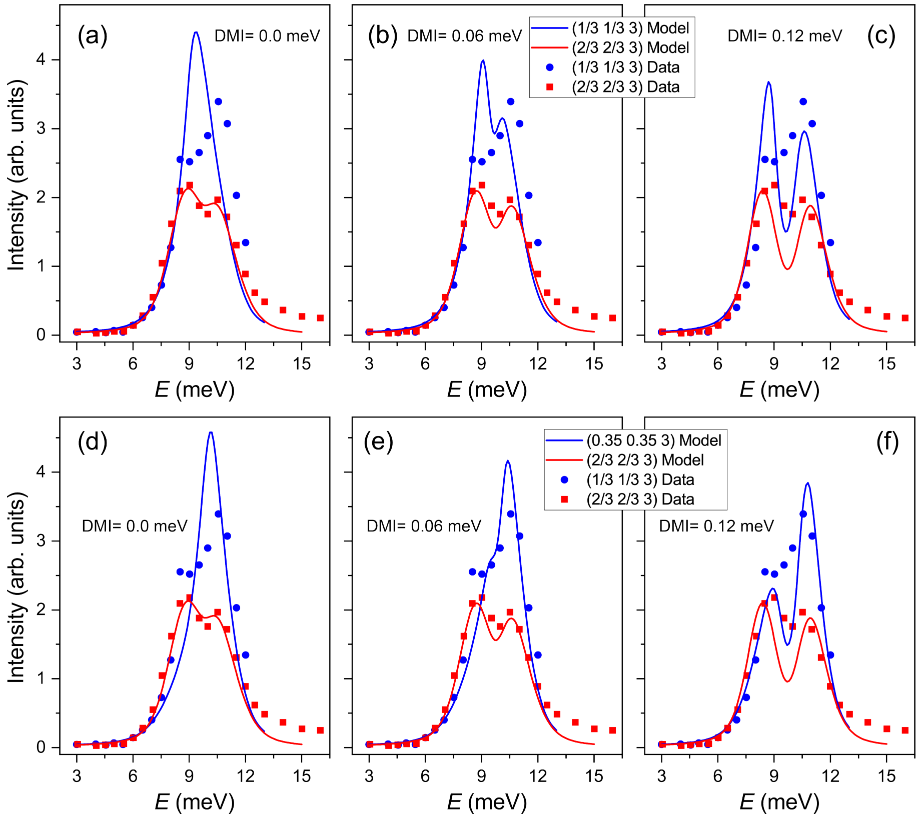


FIG. S6. Comparison of calculated spectrum with varying DMI size and experimental data from a *triple-axis* spectrometer experiment for $CrSiTe_3$ [7]. The blue (red) filled circles are experimental constant momentum scan data at $K_1$ $(\frac{1}{3},\frac{1}{3},3)$ ($K_2$ $(\frac{2}{3},\frac{2}{3},3)$), digitized from Ref.[7]. (a-c) The blue and red solid lines are calculated spectrum at $K_1$ $(\frac{1}{3},\frac{1}{3},3)$ and $K_2$ $(\frac{2}{3},\frac{2}{3},3)$, respectively for the Heisenberg Hamiltonian parameters with DMI from 0 meV to 0.12 meV as described in the text, including instrumental resolution-convolution of the experimental conditions used in Ref.[7]. (d-h) The blue and red solid lines are calculated spectrum at $K_1$ $(0.35,0.35,3)$ and $K_2$ $(\frac{2}{3},\frac{2}{3},3)$.

## VI. REINTERPRETATION OF DMI SIZE IN $CRSITE_3$

In this section, we discuss the previously published triple-axis neutron spectroscopy results of $CrSiTe_3$ [7]. As described in the main text, the spectrum at the K-point depends strongly on the shape of the resolution function. Figure S7 demonstrates how the resolution ellipses couple to magnon dispersions at the K-points and how it determines the focused and defocused regions. We assumed that the collected constant momentum scan at $K_1$ in Ref. [7] was measured in the focused region, and compare the experimental data with spectrum simulated with varying DMI in accurate resolution-convolved spin-wave calculations for $CrSiTe_3$.

Figure S6 shows the simulated spin-wave spectra for $CrSiTe_3$ [7], including the resolution calculation for the experiment using Reslib [5]. For the pin-wave calculation, we used Heisenberg spin Hamiltonian parameters ($J_1$=-1.49 meV, $J_2 = -0.15$ meV, $J_{c1} = -0.07$, $J_{c2} = -0.06$, and $D^z = -0.01$ meV) from Ref. [7] with the second n.n. DMI= 0 meV, 0.06 meV, and 0.12 meV. Figure S6 (a-c) compare the resulting simulations with the experimental data at $K_1$ $(\frac{1}{3},\frac{1}{3},3)$ and $K_2$ $(\frac{2}{3},\frac{2}{3},3)$. For the zero DMI model, the simulated constant momentum scan at $K_1$ (focused region) shows a single peak corresponding to a gapless Dirac magnon spectrum (solid blue line in Fig.S6(a)), but its line shape is narrower than data, the simulated intensity is shifted to lower energies, and it does not explain the peak splitting observed in the experimental data (blue filled circles). For non-zero DMI, the calculated spectrum opens a gap which generates two peaks, and the size of the gap increases as the strength of DMI increases. However, we note that the line shape of the simulated peaks for all the DMI values up to 0.12 meV do not match the experimental data: the intensity ratio between lower and upper magnon bands is reversed when compared to the experimental data. In practice, the measured wave vector can slightly deviate from exact K-point, $(\frac{1}{3},\frac{1}{3},3)$, or the crystal can be slighly mis-aligned. To obtain better agreement with the data, we also simulate the spectrum at $\boldsymbol{Q}= (0.35,0.35,3)$. The simulated spectrum at this wave vector better reproduces not only the measured peak intensity distribution but also line shape observed for $K_1^{\text{focus}}$. Through a qualitative comparison with experimental data, we found that DMI= 0.06 meV provides a good description of the observed peak splitting and line shape [Fig. S6(e)]. On the other hand, in the $K_2$ defocused region, the line shape is much less-sensitive to the DMI value and both 0 meV and 0.06 meV provide good agreement with the data. We note that 0.12 meV (the estimated best parameter in

Ref.[7]) does not provide good agreement with the data.

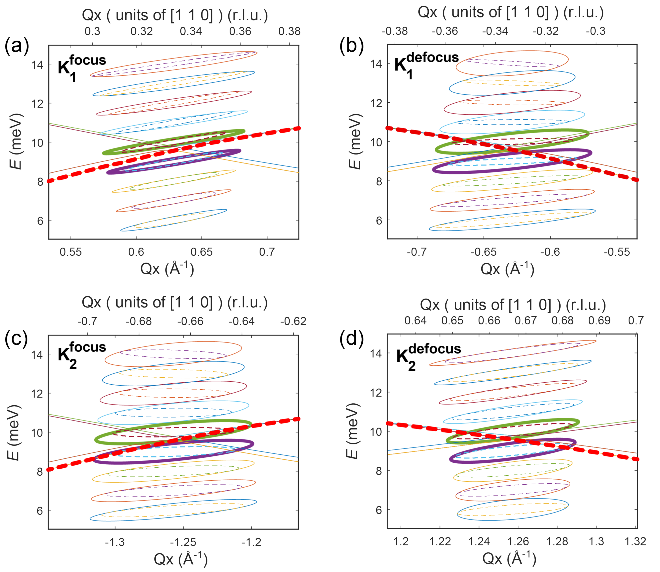


FIG. S7. Resolution ellipses and coupling to magnon dispersions for constant momentum scans at (a) $K_1^{focus}$, (b) $K_2^{defocus}$, (c) $K_1^{defocus}$, and (d) $K_2^{focus}$ for the IN8 *triple-axis* spectrometer experiment for $CrSiTe_3$ [7]. At each energy transfer plotted, the solid (dashed) ellipses correspond to the projection (section) of the resolution function onto the $\boldsymbol{Q}_x$-$E$ plane. The solid lines are magnon dispersions of $CrSiTe_3$. The red thick dashed lines and think ellipses indicate intense magnon modes and resolution functions coupled with the magnons at K-points. As a result of the coupling, the K-points are divided into 'focus' and 'defocus' regions according to whether the intense dispersion is parallel to and anti-parallel to the ellipse, respectively.


[1] O. Arnold, J. Bilheux, J. Borreguero, A. Buts, S. Campbell, L. Chapon, M. Doucet, N. Draper, R. Ferraz Leal, M. Gigg, V. Lynch, A. Markvardsen, D. Mikkelson, R. Mikkelson, R. Miller, K. Palmen, P. Parker, G. Passos, T. Perring, P. Peterson, S. Ren, M. Reuter, A. Savici, J. Taylor, R. Taylor, R. Tolchenov, W. Zhou, and J. Zikovsky, Mantid—Data analysis and visualization package for neutron scattering and $\mu$SR experiments, Nuclear Instruments and Methods in Physics Research Section A: Accelerators, Spectrometers, Detectors and Associated Equipment **764**, 156 (2014).

[2] R. Azuah, L. Kneller, Y. Qiu, P. Tregenna-Piggott, C. Brown, J. Copley, and R. Dimeo, Dave: A comprehensive software suite for the reduction, visualization, and analysis of low energy neutron spectroscopic data, J. Res. Natl. Inst. Stan. Technol. **114**, 341 (2009).

[3] R. Ewings, A. Buts, M. Le, J. Van Duijn, I. Bustinduy, and T. Perring, Horace: software for the analysis of data from single crystal spectroscopy experiments at time-of-flight neutron instruments, Nuclear Instruments and Methods in Physics Research Section A: Accelerators, Spectrometers, Detectors and Associated Equipment **834**, 132 (2016).

[4] S. Toth and B. Lake, Linear spin wave theory for single-q incommensurate magnetic structures, Journal of Physics: Condensed Matter **27**, 166002 (2015).

[5] E. Farhi, Y. Debab, and P. Willendrup, iFit: A new data analysis framework. Applications for data reduction and optimization of neutron scattering instrument simulations with McStas, Journal of Neutron Research **17**, 5 (2014).

[6] M. Popovici, On the resolution of slow-neutron spectrometers. IV. The triple-axis spectrometer resolution function, spatial effects included, Acta Crystallographica Section A **31**, 507 (1975).

[7] F. Zhu, L. Zhang, X. Wang, F. J. dos Santos, J. Song, T. Mueller, K. Schmalzl, W. F. Schmidt, A. Ivanov, J. T. Park, J. Xu, J. Ma, S. Lounis, S. Blügel, Y. Mokrousov, Y. Su, and T. Brückel, Topological magnon insulators in two-dimensional van der Waals ferromagnets $CrSiTe_3$ and $CrGeTe_3$: Toward intrinsic gap-tunability, Science Advances **7**, eabi7532 (2021).

[8] P. R. Bevington and D. K. Robinson, Data reduction and error analysis, McGraw Hill, New York (2003).

[9] L. Chen, J.-H. Chung, T. Chen, C. Duan, A. Schneidewind, I. Radelytskyi, D. J. Voneshen, R. A. Ewings, M. B. Stone, A. I. Kolesnikov, B. Winn, S. Chi, R. A. Mole, D. H. Yu, B. Gao, and P. Dai, Magnetic anisotropy in ferromagnetic $CrI_3$, Phys. Rev. B **101**, 134418 (2020).

[10] E. J. Samuelsen, R. Silberglitt, G. Shirane, and J. P. Remeika, Spin Waves in Ferromagnetic $CrBr_3$ Studied by Inelastic Neutron Scattering, Phys. Rev. B **3**, 157 (1971).

[11] D.-H. Kim, K. Kim, K.-T. Ko, J. Seo, J. S. Kim, T.-H. Jang, Y. Kim, J.-Y. Kim, S.-W. Cheong, and J.-H. Park, Giant Magnetic Anisotropy Induced by Ligand *LS* Coupling in Layered Cr Compounds, Phys. Rev. Lett. **122**, 207201 (2019).

[12] L. Chen, J.-H. Chung, M. B. Stone, A. I. Kolesnikov, B. Winn, V. O. Garlea, D. L. Abernathy, B. Gao, M. Augustin, E. J. G. Santos, and P. Dai, Magnetic Field Effect on Topological Spin Excitations in $CrI_3$, Phys. Rev. X **11**, 031047 (2021).

[13] S. A. Owerre, A first theoretical realization of honeycomb topological magnon insulator, Journal of Physics: Condensed Matter **28**, 386001 (2016).
